# Supplementary material for: Non-polynomial Worst-Case Analysis of Recursive Programs
Source: arXiv:1705.00317 source file (2017-04-30)
Supplement: Supplementary file 1 [file hongfei_appendix.tex]

%%% INFORMAL CFG.
%%We refer to the status of the program counter as a \emph{label}, and assign an initial label and a terminal label to the function body of each function call.
%%Moreover, we will have four types of labels, namely \emph{branching}, \emph{assignment}, \emph{call} and \emph{demonic} labels (cf. Figure~\ref{fig:syntax}).
%%A branching label corresponds to a conditional-branching statement indicated by the keyword `\textbf{if}' or `\textbf{while}' together with some propositional arithmetic predicate $\phi$,
%%and leads to the next label in the current function body determined by $\phi$ without change on values.
%%An assignment label corresponds to an assignment statement indicated by `$:=$' or $\mathbf{skip}$,
%%and leads to the next label right after the statement in the current function body with change of values specified by the assignment function at the right-hand-side of `$:=$'.
%%($\mathbf{skip}$ is deemed as an assignment statement that does not change values.)
%%A call label corresponds to a function call with some function name $\fn{f}$ and value-passing function, leads to the next label in the current function body, and does not change the values in the current function body.
%%Finally, a demonic label corresponds to a demonic non-deterministic statement indicated by `\textbf{if}' and `$\star$', and leads to two labels specified by the `\textbf{then}' and the `\textbf{else}' branches.
%%The detailed illustration for CFGs is as follows.

%%\smallskip
\begin{definition}[Schedulers]\label{def:scheduler}
A \emph{scheduler} (for $W$) is a function $\pi$ which maps every non-empty finite word of configurations $w_0\dots w_n$
with $w_n=(\fn{f}, \loc, \nu)\cdot w'$ being non-deterministic to a label $\loc'\in\locs{f}$ such that $(\loc,\star,\loc')\in\transitions{\fn{f}}$.
\end{definition}

%%\smallskip
\begin{remark}\label{rmk:demonicnondeterminism}
With the notion of schedulers, a scheduler can mimic any array-relevant conditional if-branches through non-determinism (indicated by $\star$) by simply making decisions according to relevant arrays at if-branches with $\star$.
In this sense, the abstraction of arrays through demonic non-determinism preserves worst-case complexity.\qed
\end{remark}

Now the semantics for our programming language follows from standard semantics in conventional programming languages (e.g., C programming language).

\noindent{\bf The Semantics.}
Given a non-terminal stack element $\mathfrak{c}$ (serving as the initial stack element) and a scheduler $\pi$, the \emph{run} $\rho(\mathfrak{c},\pi)$ is an infinite sequence
$\{w_j\}_{j\in\Nset_0}$ of configurations, initialized with $w_0=\mathfrak{c}$, inductively defined as follows.
\begin{compactitem}
%%\item \emph{Initialization:} $w_0:=\mathfrak{c}$.
%%or $w_j$ is a single letter $\sigma=(\fn{f},\lout{\fn{f}},\nu)$, for $\fn{f}\in\fnames$ and $\nu\in\Val{f}$,
\item \emph{Termination:} If $w_j=\varepsilon$  then $w_{j+1}:=\varepsilon$.

\item \emph{Inductive Step:} Assume that $w_j=(\fn{f},\loc,\nu)\cdot w'$. Then:
\begin{compactenum}
\item \emph{assignment:} if $\loc\in\alocs{f}$, $(\loc,f,\loc')$ is the only triple in $\transitions{\fn{f}}$ and $\nu'=f(\nu)$, then (i) $w_{j+1}:=(\fn{f},\loc',\nu')\cdot w'$ whenever $\loc'\ne\lout{\fn{f}}$ and
    (ii) $w_{j+1}:=w'$ otherwise;

\item  \emph{branching:} if $\loc\in\clocs{f}$ and $(\loc,\phi,\loc')$ is the only triple in $\transitions{\fn{f}}$ such that $\nu\models\phi$, then (i) $w_{j+1}:=(\fn{f},\loc',\nu)\cdot w'$
whenever $\loc'\ne\lout{\fn{f}}$ and
(ii)~$w_{j+1}:=w'$ otherwise;
\item \emph{call:} if $\loc\in\flocs{f}$ and $(\loc,(\fn{g},f),\loc')$ is the only triple in $\transitions{\fn{f}}$, then (i)~$w_{j+1}:=(\fn{g},\lin{\fn{g}},f(\nu))\cdot (\fn{f},\loc',\nu)\cdot w'$
whenever $\loc'\ne\lout{\fn{f}}$ and  (ii)~$w_{j+1}:=(\fn{g},\lin{\fn{g}},f(\nu))\cdot w'$ otherwise;
\item \emph{nondeterminism:} if $\loc\in\dlocs{f}$ and $\loc'=\pi(w_0\dots w_j)$, then (i) $w_{j+1}:=(\fn{f},\loc',\nu)\cdot w'$ whenever $\loc'\ne\lout{\fn{f}}$ and  (ii) $w_{j+1}:=w'$ otherwise.
\end{compactenum}
\end{compactitem}

%%\smallskip

With the expansion operation, it is possible to obtain a measure function by imposing constraints on a function defined at significant labels only.

In order to avoid direct manipulation of $D_{\fn{f},\loc}$'s (reachable
valuations), we further fix an invariant  w.r.t $\fn{f}^*,\phi^*$ and use it to over-approximate $D_{\fn{f},\loc}$'s.
Then we obtain the following proposition (proof in Appendix~\ref{app:propmfunc}).

%%\smallskip
\begin{proposition}\label{prop:mfunc}
Let $g$ be a function from
$\left\{(\fn{f},\loc,\nu)\mid \fn{f}\in\fnames, \loc\in\slocs{f},  \nu\in\Aval{f}\right\}$
into $[0,\infty]$.
Let $I$ be an invariant w.r.t $\fn{f}^*,\phi^*$.
Consider that for all stack elements $(\fn{f},\loc,\nu)$ such that $\loc\in\slocs{f}$ and  $\nu\models I(\fn{f},\loc)$,
the following conditions hold:
\begin{compactitem}
\item \textbf{C2':} if $\loc\in\alocs{f}$ and $(\loc,f,\loc')$ is the only triple in $\transitions{\fn{f}}$ with source label $\loc$, then  $\widehat{g}(\fn{f},\loc',f(\nu))+1\le \widehat{g}(\fn{f},\loc,\nu)$;
\item \textbf{C3':} if $\loc\in\flocs{f}$ and $(\loc,(\fn{g},f),\loc')$ is the only triple in $\transitions{\fn{f}}$ with source label $\loc$, then $1+\widehat{g}(\fn{g},\lin{\fn{g}},f(\nu))+\widehat{g}(\fn{f},\loc',\nu)\le \widehat{g}(\fn{f},\loc,\nu)$;
\item \textbf{C4':} if $\loc\in\clocs{f}$ and $(\loc, \phi,\loc_1),(\loc, \neg\phi,\loc_2)$ are namely two triples in $\transitions{\fn{f}}$ with source label $\loc$, then
$\mathbf{1}_{\nu\models\phi}\cdot \widehat{g}(\fn{f},\loc_1,\nu)+\mathbf{1}_{\nu\models\neg\phi}\cdot \widehat{g}(\fn{f},\loc_2,\nu)+1\le \widehat{g}(\fn{f},\loc,\nu)$\enskip;
\item \textbf{C5':} if $\loc\in\dlocs{f}$ and $(\loc, \star,\loc_1),(\loc, \star,\loc_2)$ are namely two triples in $\transitions{\fn{f}}$ with source label $\loc$, then
$\max\{\widehat{g}(\fn{f},\loc_1,\nu), \widehat{g}(\fn{f},\loc_2,\nu)\}+1\le \widehat{g}(\fn{f},\loc,\nu)$.
\end{compactitem}
Then $\widehat{g}$ is a measure function w.r.t $\fn{f}^*,\phi^*$.
\end{proposition}

Note that conditions C2'-C5' essentially specify constraints on $g$.
This allows an algorithm to synthesize a measure function only at significant labels.

%%%%%%%%%%%%%
In this section we explain how our sound algorithm is applicable for termination
analysis of recursive programs as well as to obtain non-trivial worst-case
bounds.

\vspace{-1.5em}
\subsection{Termination of Recursive Programs}\label{sect:termexp}
\vspace{-0.8em}
For termination of recursive programs we consider two examples,
described below.

%%\smallskip
\noindent{\em Example 1: Walk on Two-Dimensional Plane.}
We first consider a simple deterministic walk on a two-dimensional plane, until a boundary
is reached. We consider the walk as a recursive procedure given in the left part of Fig.~\ref{fig:termexp}.
With a linear template ($d=1$ and $\mathrm{op}$ irrelevant for the input parameters), our algorithm synthesizes a linear measure function.

\lstset{language=prog}
\lstset{tabsize=3}
\newsavebox{\prograndwalk}
\begin{lrbox}{\prograndwalk}
\begin{lstlisting}[mathescape]
$\mathsf{randwalk}(i, j)$ {
if $2*i+3*j\le 100$
  then
    $i:=i-1$;
    $j:=j+1$;
    $\mathsf{randwalk}(i,j)$
  else skip
fi }

\end{lstlisting}
\end{lrbox}

\lstset{language=prog}
\lstset{tabsize=3}
\newsavebox{\prognestedloop}
\begin{lrbox}{\prognestedloop}
\begin{lstlisting}[mathescape]
| $\mathsf{nestedloop}(i, j, m, n)$ {
| if $i\le m$ then
|   if $j\le n$ then $j:=j+1$
|   else $i:=i+1$; $j:=0$
|   fi;
|   $\mathsf{nestedloop}(i,j,m,n)$
|   else skip
| fi }
\end{lstlisting}
\end{lrbox}

\begin{figure}
\centering
\usebox{\prograndwalk}
\usebox{\prognestedloop}
\caption{Programs for Section~\ref{sect:termexp}}
\label{fig:termexp}
\end{figure}

%%\smallskip
\noindent{\em Example 2: Nested Loop.}
We consider a recursive procedure that implements a nested loop, given in the
right part of Fig.~\ref{fig:termexp}, and
with a quadratic template ($d=2$ and $\mathrm{op}$ irrelevant for the input parameters), our algorithm synthesizes a quadratic measure
function.

The above two examples are simple representative of recursive programs, and our algorithm can synthesize linear and quadratic bounds for
termination of recursive programs.

\vspace{-1.5em}
\subsection{Non-trivial Worst-Case Bounds}
\vspace{-0.8em}
%%%%%%%%%%%%%%
